# Supplementary material for: Fine-grained Species Recognition with Privileged Pooling: Better Sample Efficiency Through Supervised Attention
Source: arXiv:2003.09168 source file (2023-08-04)
Supplement: Supplementary file 1 [file cct_results_supplementary.tex]

\begin{tabular}{llrrrrrrrr}
\toprule
    & dataset & \multicolumn{4}{l}{cct20\_cis} & \multicolumn{4}{l}{cct20\_trans} \\
    & {} & \multicolumn{2}{l}{Acc} & \multicolumn{2}{l}{Acc\_class} & \multicolumn{2}{l}{Acc} & \multicolumn{2}{l}{Acc\_class} \\
    & Full &     False & True  &     False & True  &       False & True  &     False & True  \\
Pool & Model &           &       &           &       &             &       &           &       \\
\midrule
Avg & MultiTask &      72.2 &  76.4 &      59.5 &  65.8 &        65.6 &  67.2 &      42.6 &  50.0 \\
    & Pool &      71.4 &  73.6 &      57.0 &  59.8 &        65.1 &  66.1 &      42.0 &  43.6 \\
    & PrPool &      80.3 &  82.1 &      66.8 &  73.3 &        72.0 &  68.5 &      55.1 &  60.2 \\
    & PrPool- &      81.0 &  83.5 &      69.4 &  70.3 &        70.6 &  72.3 &      52.7 &  54.8 \\
    & S3N &      75.2 &  75.5 &      61.7 &  66.7 &        64.2 &  70.6 &      40.2 &  50.9 \\
    & WSDAN &      71.7 &  75.7 &      50.8 &  64.9 &        60.3 &  62.5 &      33.5 &  42.5 \\
    & WSDAN- &      72.9 &  76.2 &      52.2 &  63.9 &        62.6 &  61.4 &      34.7 &  42.4 \\
Cov & Pool &      74.3 &  81.4 &      59.8 &  69.3 &        67.2 &  70.1 &      41.9 &  43.8 \\
    & PrPool &      68.8 &  75.9 &      46.7 &  56.3 &        64.8 &  70.5 &      41.2 &  49.5 \\
    & PrPool- &      76.7 &  82.9 &      57.0 &  69.9 &        68.5 &  75.0 &      42.8 &  51.6 \\
\bottomrule
\end{tabular}
